# Supplementary material for: Current-assisted Raman activation of the Higgs mode in superconductors
Source: arXiv:2001.08091 source file (2020-06-17)
Supplement: Supplementary file 1 [file supplement.pdf]

# Supplemental material: Current-assisted Raman activation of the Higgs mode in superconductors


Matteo Puviani,[1] Lukas Schwarz,[1] Xiao-Xiao Zhang,[2] Stefan Kaiser,[1,3] and Dirk Manske[1,*]

[1] *Max Planck Institute for Solid State Research, 70569 Stuttgart, Germany*

[2] *Department of Physics and Astronomy & Stewart Blusson Quantum Matter Institute, University of British Columbia, Vancouver, Canada BC V6T 1Z4*

[3] *4th Physics Institute and Research Center SCoPE, University of Stuttgart, 70569 Stuttgart, Germany*



(Dated: June 17, 2020)


## I. EVALUATION OF THE INFRARED DIAGRAM

The response of the diagram in Fig. 1(a) from the main text is proportional to

$$R(\boldsymbol{Q},\Omega) \propto \boldsymbol{Q}\boldsymbol{A}\left|\chi^{\mathrm{H}}_{\mathrm{jj}}(\boldsymbol{Q},\Omega)\right| . \tag{1}$$

In particular, the susceptibility for the current-current interaction vertices (each with interaction term $j_{\boldsymbol{k}}\tau_0$) can be expressed as

$$\chi^{\mathrm{H}}_{\mathrm{jj}}(\boldsymbol{q},\Omega) = H(\boldsymbol{q},\Omega)\chi^{2}_{\mathrm{j1}}(\boldsymbol{q},\Omega) , \tag{2}$$

with the dressed Higgs propagator calculated by means of a RPA summation [1] as $H(\boldsymbol{q},\Omega) = -\left(2/V + \chi_{11}(\boldsymbol{q},\Omega)\right)^{-1}$, where $\chi_{11}(\boldsymbol{q},\Omega)$ is the $\tau_1 - \tau_1$ bubble susceptibility and $V$ the pairing strength. Therefore, we can rewrite the expression in (2) as

$$\chi^{\mathrm{H}}_{\mathrm{jj}}(\boldsymbol{q},\Omega) = -\frac{\chi^{2}_{\mathrm{j1}}(\boldsymbol{q},\Omega)}{2/V + \chi_{11}(\boldsymbol{q},\Omega)} . \tag{3}$$

The bubble susceptibilities appearing in this expression are calculated as

$$\chi_{11}(\boldsymbol{q},\mathrm{i}\omega_n) = \sum_{\boldsymbol{k}} f^2_{\boldsymbol{k}} \frac{1}{\beta}\sum_{\mathrm{i}\nu_m} \mathrm{Tr}\left[G(\boldsymbol{k},\mathrm{i}\nu_m)\tau_1 G(\boldsymbol{k}+\boldsymbol{q},\mathrm{i}\nu_m+\mathrm{i}\omega_n)\tau_1\right] , \tag{4}$$

$$\chi_{\mathrm{j1}}(\boldsymbol{q},\mathrm{i}\omega_n) = \sum_{\boldsymbol{k}} f_{\boldsymbol{k}} j_{\boldsymbol{k}} \frac{1}{\beta}\sum_{\mathrm{i}\nu_m} \mathrm{Tr}\left[G(\boldsymbol{k},\mathrm{i}\nu_m)\tau_0 G(\boldsymbol{k}+\boldsymbol{q},\mathrm{i}\nu_m+\mathrm{i}\omega_n)\tau_1\right] , \tag{5}$$

where $f_{\boldsymbol{k}}$ is the gap symmetry form factor, $j_{\boldsymbol{k}}$ is the gradient of the energy projected onto the direction of the light polarization, $\tau_i$ with $i = 1, 2, 3$ are the Pauli matrices and $\tau_0$ is the identity matrix. Moreover, we use $\mathrm{i}\nu_m$ for the fermion frequency and $\mathrm{i}\omega_n$ for the boson frequency, where the Nambu Green's function with Matsubara frequencies $\mathrm{i}\nu_m$ is given by

$$G(\boldsymbol{k},\mathrm{i}\nu_m) = \frac{1}{(\mathrm{i}\nu_m)^2 - E^2_{\boldsymbol{k}}} \cdot \begin{pmatrix} \mathrm{i}\nu_m + \epsilon_{\boldsymbol{k}} & \Delta_{\boldsymbol{k}} \\ \Delta_{\boldsymbol{k}} & \mathrm{i}\nu_m - \epsilon_{\boldsymbol{k}} \end{pmatrix} . \tag{6}$$

Solving analytically the Matsubara summation we get the forms

$$\begin{aligned} \chi_{11}(\boldsymbol{q},\mathrm{i}\omega_n) = \sum_{\boldsymbol{k}} f^2_{\boldsymbol{k}} \iint \mathrm{d}\omega_1\,\mathrm{d}\omega_2\, &\frac{\Delta_{\boldsymbol{k}}\Delta_{\boldsymbol{k}+\boldsymbol{q}} + \omega_1\omega_2 - \epsilon_{\boldsymbol{k}}\epsilon_{\boldsymbol{k}+\boldsymbol{q}}}{2E_{\boldsymbol{k}}E_{\boldsymbol{k}+\boldsymbol{q}}} \frac{n_{\mathrm{F}}(\omega_1) - n_{\mathrm{F}}(\omega_2)}{\omega_1 - \omega_2 + \mathrm{i}\omega_n} \\ &\times \left[\delta(\omega_1 - E_{\boldsymbol{k}}) - \delta(\omega_1 + E_{\boldsymbol{k}})\right]\left[\delta(\omega_2 - E_{\boldsymbol{k}+\boldsymbol{q}}) - \delta(\omega_2 + E_{\boldsymbol{k}+\boldsymbol{q}})\right] , \end{aligned} \tag{7}$$

$$\begin{aligned} \chi_{\mathrm{j1}}(\boldsymbol{q},\mathrm{i}\omega_n) = \sum_{\boldsymbol{k}} j_{\boldsymbol{k}} f_{\boldsymbol{k}} \iint \mathrm{d}\omega_1\,\mathrm{d}\omega_2\, &\frac{\Delta_{\boldsymbol{k}}\omega_2 + \Delta_{\boldsymbol{k}+\boldsymbol{q}}\omega_1}{2E_{\boldsymbol{k}}E_{\boldsymbol{k}+\boldsymbol{q}}} \frac{n_{\mathrm{F}}(\omega_1) - n_{\mathrm{F}}(\omega_2)}{\omega_1 - \omega_2 + i\omega_n} \\ &\times \left[\delta(\omega_1 - E_{\boldsymbol{k}}) - \delta(\omega_1 + E_{\boldsymbol{k}})\right]\left[\delta(\omega_2 - E_{\boldsymbol{k}+\boldsymbol{q}}) - \delta(\omega_2 + E_{\boldsymbol{k}+\boldsymbol{q}})\right] . \end{aligned} \tag{8}$$


* d.manske@fkf.mpg.de

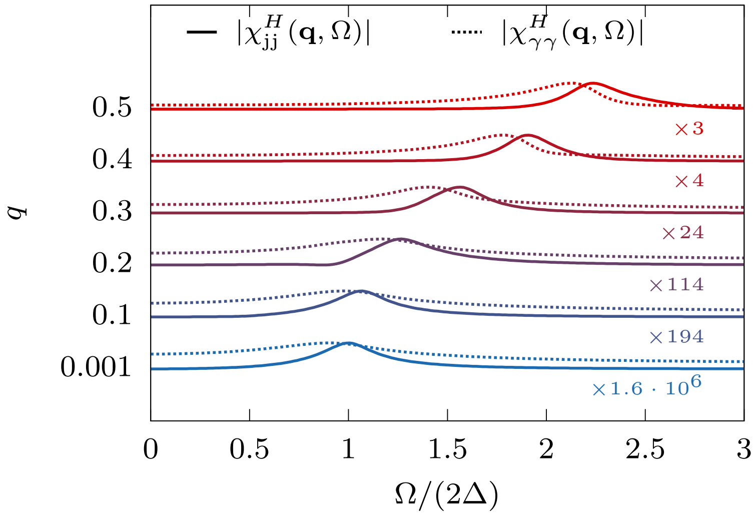


Figure 1. Evaluation of the Higgs susceptibility using the infrared diagram in Fig. 1(a) of the main text compared to the Raman-like diagram in Fig. 1(b). For small $q$, the infrared diagram is negligible. For increasing values of $q$, the diagram gets finite but shifted to higher energies, reflecting the dispersion of the Higgs mode.

The susceptibilities in (3) are obtained with the analytic continuation $\mathrm{i}\omega_n \to \Omega + \mathrm{i}\delta$ from these expressions. In the limit $\boldsymbol{q} \to 0$, the susceptibility $\chi_{\mathrm{j}1}(\boldsymbol{q}=0,\Omega) = 0$ vanishes. An evaluation for increasing $\boldsymbol{q}$ is shown in Fig. 1 compared to the contribution from the Raman-like diagram (see Sec. II). For small $\boldsymbol{q}$, the infrared contribution is still negligible. For large $\boldsymbol{q}$, the contribution gets comparable to the Raman-like contribution, however is no longer peaked at $\Omega = 2\Delta$ but shifted to higher energies. This reflects the dispersion of the Higgs mode for finite $\boldsymbol{q}$. Thus, the infrared diagram cannot explain a resonance at $\Omega = 2\Delta$ as either its contribution is negligible for small $\boldsymbol{q}$ or not peaked at $\Omega = 2\Delta$ for large $\boldsymbol{q}$.

## II. EVALUATION OF THE RAMAN-LIKE DIAGRAM

The susceptibility for the diagram in Fig. 1(b) of the main text is given by

$$\chi^{\mathrm{H}}_{\gamma\gamma}(\boldsymbol{q},\Omega) = H(\boldsymbol{q},\Omega)\chi^2_{\gamma 1}(\boldsymbol{q},\Omega)\,, \tag{9}$$

with

$$\chi_{\gamma 1}(\boldsymbol{q},\mathrm{i}\omega_n) = \sum_{\boldsymbol{k}} f_{\boldsymbol{k}}\gamma_{\boldsymbol{k}}\frac{1}{\beta}\sum_{\mathrm{i}\nu_m}\mathrm{Tr}\left[G(\boldsymbol{k},\mathrm{i}\nu_m)\tau_3 G(\boldsymbol{k}+\boldsymbol{q},\mathrm{i}\nu_m+\mathrm{i}\omega_n)\tau_1\right]\,. \tag{10}$$

Solving analytically the Matsubara summation, we get the form

$$\chi_{\gamma 1}(\boldsymbol{q},\mathrm{i}\omega_n) = \sum_{\boldsymbol{k}}\gamma_{\boldsymbol{k}} f_{\boldsymbol{k}}\iint_{-\infty}^{+\infty}\frac{\epsilon_{\boldsymbol{k}}\Delta_{\boldsymbol{k}+\boldsymbol{q}}+\epsilon_{\boldsymbol{k}+\boldsymbol{q}}\Delta_{\boldsymbol{k}}}{2E_{\boldsymbol{k}}E_{\boldsymbol{k}+\boldsymbol{q}}}\cdot\frac{n_{\mathrm{F}}(\omega_1)-n_{\mathrm{F}}(\omega_2)}{\omega_1-\omega_2+\mathrm{i}\omega_n}$$
$$\times\left[\delta(\omega_1-E_{\boldsymbol{k}})-\delta(\omega_1+E_{\boldsymbol{k}})\right]\left[\delta(\omega_2-E_{\boldsymbol{k}+\boldsymbol{q}})-\delta(\omega_2+E_{\boldsymbol{k}+\boldsymbol{q}})\right]\,. \tag{11}$$

A calculation of the susceptibility in real frequency spectrum for varying values of $\boldsymbol{q}$ is shown in Fig. 1. An evaluation in real frequency spectrum and in the limit $\boldsymbol{q} \to 0$ yields

$$\chi^{\mathrm{H}}_{\gamma\gamma}(\Omega) = -2\frac{\sum_{\boldsymbol{k}}\frac{\gamma_{\boldsymbol{k}} f^2_{\boldsymbol{k}}\epsilon_{\boldsymbol{k}}\Delta}{E_{\boldsymbol{k}}(4E^2_{\boldsymbol{k}}-\Omega^2)}}{1/V-\sum_{\boldsymbol{k}}\frac{2\epsilon^2_{\boldsymbol{k}} f^2_{\boldsymbol{k}}}{E_{\boldsymbol{k}}(4E^2_{\boldsymbol{k}}-\Omega^2)}}\,. \tag{12}$$

This expression is always nonzero. We can compare the susceptibility with the solution of $\delta\Delta$ from the pseudospin analysis in the next section. Inserting Eq. (31) with just the $\gamma^{A^2}_{\boldsymbol{k}}(s)$ term, written as $\gamma^{A^2}_{\boldsymbol{k}}(s) = \partial^2_{\boldsymbol{k}}\epsilon_{\boldsymbol{k}} e^2 A(s)^2$, into the

gap equation, we obtain for $s = \mathrm{i}\Omega$

$$\delta\Delta(\Omega) = V \sum_{\boldsymbol{k}} \frac{2\epsilon_{\boldsymbol{k}}^2 f_{\boldsymbol{k}}^2}{E_{\boldsymbol{k}}(4E_{\boldsymbol{k}}^2 - \Omega^2)} \delta\Delta(\Omega) - V \sum_{\boldsymbol{k}} \frac{\partial_{\boldsymbol{k}}^2 \epsilon_{\boldsymbol{k}} f_{\boldsymbol{k}}^2 \epsilon_{\boldsymbol{k}} \Delta e^2 A(\Omega)^2}{E_{\boldsymbol{k}}(4E_{\boldsymbol{k}}^2 - \Omega^2)} . \tag{13}$$

Solving for $\delta\Delta$ yields just the result (12). The linear pseudospin analysis is therefore equivalent to the Raman-like diagram.

## III. PSEUDOSPIN ANALYSIS

We use the BCS Hamiltonian and the time-dependent gap equation $\Delta_{\boldsymbol{k}}(t) = \Delta(t) f_{\boldsymbol{k}}$ in the Anderson pseudospin formalism [2]

$$H = \sum_{\boldsymbol{k}} \boldsymbol{b}_{\boldsymbol{k}} \boldsymbol{\sigma}_{\boldsymbol{k}} , \qquad \Delta(t) = V \sum_{\boldsymbol{k}} f_{\boldsymbol{k}} \left\langle \sigma_{\boldsymbol{k}}^x \right\rangle (t) , \tag{14}$$

where the pseudospins are defined as $\boldsymbol{\sigma}_{\boldsymbol{k}} = \frac{1}{2} \Psi_{\boldsymbol{k}}^\dagger \boldsymbol{\tau} \Psi_{\boldsymbol{k}}$, with the Nambu-Gorkov spinor $\Psi_{\boldsymbol{k}}^\dagger = \left( c_{\boldsymbol{k}\uparrow}^\dagger, \ c_{-\boldsymbol{k}\downarrow} \right)$ and $\boldsymbol{\tau}$ the vector of Pauli matrices. The pairing strength is given by $V$ and the gap symmetry is described by the function $f_{\boldsymbol{k}}$. Please note that in equilibrium the gap is assumed to be real and we neglect also the induced imaginary part in the time-evolution as its dynamics simply follows the driving without additional features and is therefore unimportant for the following discussion. In equilibrium, all the pseudospins are aligned parallel to the pseudomagnetic field, such that the expectation values for $T = 0$ read

$$\left\langle \sigma_{\boldsymbol{k}}^x \right\rangle = \frac{\Delta f_{\boldsymbol{k}}}{2E_{\boldsymbol{k}}} , \qquad \left\langle \sigma_{\boldsymbol{k}}^y \right\rangle = 0 , \qquad \left\langle \sigma_{\boldsymbol{k}}^z \right\rangle = -\frac{\epsilon_{\boldsymbol{k}}}{2E_{\boldsymbol{k}}} . \tag{15}$$

We use the following ansatz to describe the time-evolution of the pseudospins for small perturbations

$$\left\langle \sigma_{\boldsymbol{k}}^x \right\rangle (t) = \left\langle \sigma_{\boldsymbol{k}}^x \right\rangle + x_{\boldsymbol{k}}(t) , \qquad \left\langle \sigma_{\boldsymbol{k}}^y \right\rangle (t) = \left\langle \sigma_{\boldsymbol{k}}^y \right\rangle + y_{\boldsymbol{k}}(t) , \qquad \left\langle \sigma_{\boldsymbol{k}}^z \right\rangle (t) = \left\langle \sigma_{\boldsymbol{k}}^z \right\rangle + z_{\boldsymbol{k}}(t) , \tag{16}$$

and

$$\Delta(t) = \Delta + \delta\Delta(t) \tag{17}$$

with $x_{\boldsymbol{k}}(t), y_{\boldsymbol{k}}(t), z_{\boldsymbol{k}}(t), \delta\Delta(t) \ll 1$. The coupling to the light field $\boldsymbol{A}(t) = \boldsymbol{A}_0 \sin(\Omega t)$ and the supercurrent induced momentum $\boldsymbol{Q}$ is incorporated with the usual minimal coupling $\epsilon_{\boldsymbol{k}} \to \epsilon_{\boldsymbol{k} - e\boldsymbol{A}(t) - \boldsymbol{Q}}$, such that the pseudomagnetic field reads

$$\boldsymbol{b}_{\boldsymbol{k}}^\top(t) = \left( -2\Delta_{\boldsymbol{k}}(t), \ 0, \ \epsilon_{\boldsymbol{k} - e\boldsymbol{A}(t) - \boldsymbol{Q}} + \epsilon_{\boldsymbol{k} + e\boldsymbol{A}(t) + \boldsymbol{Q}} \right) . \tag{18}$$

The $z$-component of the pseudomagnetic field can be expanded in powers of $A_0$

$$b_{\boldsymbol{k}}^z(t) = 2\epsilon_{\boldsymbol{k}} + \gamma_{\boldsymbol{k}}^{A^2}(t) + \gamma_{\boldsymbol{k}}^{AQ}(t) + \gamma_{\boldsymbol{k}}^{Q^2} + \mathcal{O}(A_0^3) , \tag{19}$$

with

$$\gamma_{\boldsymbol{k}}^{A^2}(t) = e^2 \sum_{ij} \partial_{ij}^2 \epsilon_{\boldsymbol{k}} A_i(t) A_j(t) , \qquad \gamma_{\boldsymbol{k}}^{AQ}(t) = 2e \sum_{ij} \partial_{ij}^2 \epsilon_{\boldsymbol{k}} A_i(t) Q_j , \qquad \gamma_{\boldsymbol{k}}^{Q^2} = \sum_{ij} \partial_{ij}^2 \epsilon_{\boldsymbol{k}} Q_i Q_j . \tag{20}$$

The term $\propto \sum_i \partial_i \epsilon_{\boldsymbol{k}}$ vanishes due to particle-hole symmetry. For isotropic band dispersion and under summation over all momentum space, we simplify the derivative of the dispersion by expanding in powers of the dispersion [3]. W obtain

$$\gamma_{\boldsymbol{k}}^{A^2}(t) \approx e^2 A_0^2(t)(\alpha_0 + \alpha_1 \epsilon_{\boldsymbol{k}}) , \qquad \gamma_{\boldsymbol{k}}^{AQ}(t) \approx 2eA_0(t)Q(\alpha_0 + \alpha_1 \epsilon_{\boldsymbol{k}}) , \qquad \gamma_{\boldsymbol{k}}^{Q^2} \approx Q^2(\alpha_0 + \alpha_1 \epsilon_{\boldsymbol{k}}) , \tag{21}$$

where $\alpha_i$ are expansion coefficients. The Bloch equations $\partial_t \left\langle \boldsymbol{\sigma}_{\boldsymbol{k}} \right\rangle (t) = \boldsymbol{b}_{\boldsymbol{k}}(t) \times \left\langle \boldsymbol{\sigma}_{\boldsymbol{k}} \right\rangle (t)$, neglecting higher orders in the deviations, read

$$\dot{x}_{\boldsymbol{k}}(t) = -2\epsilon_{\boldsymbol{k}} y_{\boldsymbol{k}}(t) , \tag{22}$$

$$\dot{y}_{\boldsymbol{k}}(t) = 2\epsilon_{\boldsymbol{k}} x_{\boldsymbol{k}}(t) + 2\Delta f_{\boldsymbol{k}} z_{\boldsymbol{k}}(t) + \frac{f_{\boldsymbol{k}}}{E_{\boldsymbol{k}}} \left( \frac{\Delta}{2} \left( \gamma_{\boldsymbol{k}}^{A^2}(t) + \gamma_{\boldsymbol{k}}^{AQ}(t) + \gamma_{\boldsymbol{k}}^{Q^2} \right) - \epsilon_{\boldsymbol{k}} \delta\Delta(t) \right) , \tag{23}$$

$$\dot{z}_{\boldsymbol{k}}(t) = -2\Delta f_{\boldsymbol{k}} y_{\boldsymbol{k}}(t) . \tag{24}$$

We apply a Laplace transform from time $t$ to complex frequency $s$ to obtain algebraic equations

$$
\begin{aligned}
s x_{\boldsymbol{k}}(s) &= -2\epsilon_{\boldsymbol{k}} y_{\boldsymbol{k}}(s)\,, && (25)\\
s y_{\boldsymbol{k}}(s) &= 2\epsilon_{\boldsymbol{k}} x_{\boldsymbol{k}}(s) + 2\Delta f_{\boldsymbol{k}} z_{\boldsymbol{k}}(s) + \frac{f_{\boldsymbol{k}}}{E_{\boldsymbol{k}}}\left(\frac{\Delta}{2}\left(\gamma_{\boldsymbol{k}}^{A^2}(s) + \gamma_{\boldsymbol{k}}^{AQ}(s) + \gamma_{\boldsymbol{k}}^{Q^2}(s)\right) - \epsilon_{\boldsymbol{k}}\delta\Delta(s)\right)\,, && (26)\\
s z_{\boldsymbol{k}}(s) &= -2\Delta f_{\boldsymbol{k}} y_{\boldsymbol{k}}(s)\,, && (27)
\end{aligned}
$$

where

$$
\begin{aligned}
\gamma_{\boldsymbol{k}}^{A^2}(s) &= e^2 A_0^2(\alpha_0 + \alpha_1\epsilon_{\boldsymbol{k}})\frac{2\Omega^2}{s(4\Omega^2 + s^2)}\,, && (28)\\
\gamma_{\boldsymbol{k}}^{AQ}(s) &= 2eA_0Q(\alpha_0 + \alpha_1\epsilon_{\boldsymbol{k}})\frac{\Omega}{\Omega^2 + s^2}\,, && (29)\\
\gamma_{\boldsymbol{k}}^{Q^2}(s) &= Q^2(\alpha_0 + \alpha_1\epsilon_{\boldsymbol{k}})\frac{1}{s}\,. && (30)
\end{aligned}
$$

The solution for $x_{\boldsymbol{k}}(t)$ reads

$$
x_{\boldsymbol{k}}(s) = \frac{\epsilon_{\boldsymbol{k}} f_{\boldsymbol{k}}\left(2\epsilon_{\boldsymbol{k}}\delta\Delta(s) - \Delta\left(\gamma_{\boldsymbol{k}}^{A^2}(s) + \gamma_{\boldsymbol{k}}^{AQ}(s) + \gamma_{\boldsymbol{k}}^{Q^2}(s)\right)\right)}{E_{\boldsymbol{k}}(4E_{\boldsymbol{k}}^2 + s^2)}\,. \tag{31}
$$

Substituting this expression into the gap equation and solving for $\delta\Delta(s)$, one finds

$$
\delta\Delta(s) = \frac{1}{2}\alpha_1\Delta\left(e^2A_0^2\frac{2\Omega^2}{s(4\Omega^2+s^2)} + 2eA_0Q\frac{\Omega}{\Omega^2+s^2} + Q^2\frac{1}{s}\right)\left(1 - \frac{1}{\lambda\int \mathrm{d}\varphi f^2(4\Delta^2f^2+s^2)F(s,\varphi)}\right)\,, \tag{32}
$$

where

$$
F(s,\varphi) = \int_{-\epsilon_{\mathrm{c}}}^{\epsilon_{\mathrm{c}}} \frac{1}{2E(4E^2+s^2)}\,\mathrm{d}\epsilon = \frac{1}{s\sqrt{4\Delta^2f^2+s^2}}\sinh^{-1}\left(\frac{s}{2\Delta|f|}\right)\,. \tag{33}
$$

Here, we replace the momentum sum with an integral

$$
V\sum_{\boldsymbol{k}} \to \lambda\int_{-\epsilon_{\mathrm{c}}}^{\epsilon_{\mathrm{c}}}\mathrm{d}\epsilon\int_0^{2\pi}\mathrm{d}\varphi \tag{34}
$$

assuming $\epsilon_{\boldsymbol{k}} = \epsilon(|\boldsymbol{k}|)$ and $f_{\boldsymbol{k}} = f(\varphi)$ and using $\lambda = VD(\epsilon_{\mathrm{F}})$, where the density of states $D(\epsilon_{\mathrm{F}})$ is assumed to be constant near the Fermi energy. There are three contributions which determine the dynamics of the gap, resulting from the terms $\gamma_{\boldsymbol{k}}^{A^2}(t)$, $\gamma_{\boldsymbol{k}}^{AQ}(t)$, $\gamma_{\boldsymbol{k}}^{Q^2}$. Thus we write

$$
\delta\Delta(s) = \delta\Delta_{A^2}(s) + \delta\Delta_{AQ}(s) + \delta\Delta_{Q^2}(s)\,. \tag{35}
$$

The solution in time domain is obtained by an inverse Laplace transform, where the Bromwich integral

$$
\delta\Delta(t) = \frac{1}{2\pi\mathrm{i}}\int_{\gamma-\mathrm{i}\infty}^{\gamma+\mathrm{i}\infty}\mathrm{e}^{st}\delta\Delta(s)\,\mathrm{d}s \tag{36}
$$

has to be evaluated for $\gamma\in\mathbb{R}$ larger than any poles of the integrand. The integration can be extended into a closed loop contour integral in the complex plane as shown in Fig. 2. The contribution in the long-time limit consisting of the driven oscillations at which we are interested in, can be obtained by evaluating the residues for the poles. For $\delta\Delta_{A^2}(s)$ we have

$$
\begin{aligned}
\mathrm{Res}_0(\mathrm{e}^{st}\delta\Delta_{A^2}(s)) &= \frac{1}{4}\alpha_1\Delta e^2A_0^2\left(1 - \frac{1}{\lambda\int\mathrm{d}\varphi f^2}\right)\,, && (37)\\
\mathrm{Res}_{\pm2\mathrm{i}\Omega}(\mathrm{e}^{st}\delta\Delta_{A^2}(s)) &= \frac{1}{8}\alpha_1\Delta e^2A_0^2\left(\mathrm{e}^{\pm2\mathrm{i}\Omega} - \frac{\Omega\mathrm{e}^{\pm2\mathrm{i}\Omega}}{\lambda\int\mathrm{d}\varphi f^2\sqrt{\Delta^2f^2-\Omega^2}\sin^{-1}\left(\frac{\Omega}{\Delta|f|}\right)}\right)\,. && (38)
\end{aligned}
$$

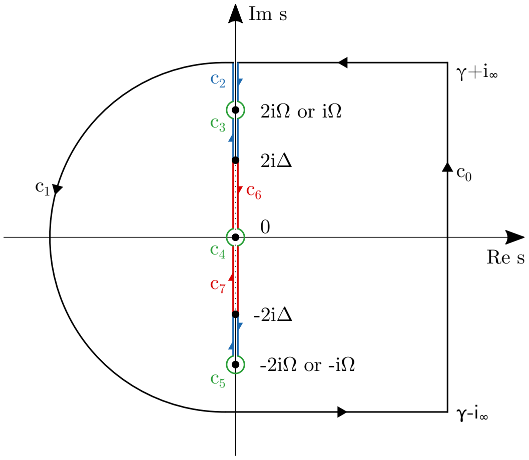


Figure 2. Bromwich integral from Eq. (36) extended into a closed loop contour integral in the complex plane. There is a continuous line of branch points at $s = \pm 2\mathrm{i}\Delta f$ (depending on $f$) and poles at $s = 0, \pm 2\mathrm{i}\Omega$ for $\delta\Delta_{A^2}$, at $s = \pm\mathrm{i}\Omega$ for $\delta\Delta_{AQ}$, and at $s = 0$ for $\delta\Delta_{Q^2}$.

An evaluation of the residues for the poles in $\delta\Delta_{AQ}(s)$ yields

$$\mathrm{Res}_{\pm\mathrm{i}\Omega}(\mathrm{e}^{st}\delta\Delta_{AQ}(s)) = \frac{1}{2}\alpha_1 \Delta e A_0 Q \left( \mp \mathrm{i}\mathrm{e}^{\pm\mathrm{i}\Omega} \mp \frac{\mathrm{i}\Omega\mathrm{e}^{\pm\mathrm{i}\Omega}}{\lambda \int \mathrm{d}\varphi f^2 \sqrt{4\Delta^2 f^2 - \Omega^2} \sin^{-1}\left(\frac{\Omega}{2\Delta|f|}\right)} \right). \tag{39}$$

The expression $\delta\Delta_{Q^2}(s)$ just adds an offset, which is not interesting for our discussion. Combining the expressions, we find

$$\delta\Delta_{A^2}(t) = \alpha_1 \Delta e^2 A_0^2 \left( \frac{1}{2}\sin(\Omega t)^2 - \frac{1}{4\lambda \int \mathrm{d}\varphi f^2} - \frac{\Omega\cos(2\Omega t)}{4\lambda \int \mathrm{d}\varphi f^2 \sqrt{\Delta^2 f^2 - \Omega^2} \sin^{-1}\left(\frac{\Omega}{\Delta|f|}\right)} \right), \tag{40}$$

$$\delta\Delta_{AQ}(t) = \alpha_1 \Delta e A_0 Q \left( \sin(\Omega t) + \frac{\Omega \sin(\Omega t)}{\lambda \int \mathrm{d}\varphi f^2 \sqrt{4\Delta^2 f^2 - \Omega^2} \sin^{-1}\left(\frac{\Omega}{2\Delta|f|}\right)} \right). \tag{41}$$

As shown in the main text in Fig. 2, the $A^2$ driving leads to a $2\Omega$ oscillation of the order parameter, which resonates at $2\Omega = 2\Delta$, while the $AQ$ driving term leads to a $\Omega$ oscillation, resonating at $\Omega = 2\Delta$. To account for the numerical divergence and include experimental broadening, we replaced $\Omega \to \Omega + 0.05\mathrm{i}$. Furthermore, the relative height of the $A^2$ and $QA$ term is compared by scaling $\delta\Delta_{AQ}$ with $4Q/(eA_0)$ using the constant amplitude $A_0 = E_0/\Omega = 1.67 \cdot 10^{-11}\,\mathrm{Vs\,cm^{-1}}$ with $E_0 = 20\,\mathrm{Vcm^{-1}}$, $\Omega = 1.2\,\mathrm{Thz}$ and $\Delta = 5\,\mathrm{meV}$ of the experiment [4]. We use different values $Q \in [0.25Q_c, 0.5Q_c, 0.75Q_c, Q_c]$ for varying current strength with the critical current $j = 3.7 \cdot 10^6\,\mathrm{A/cm^2}$, which leads to $4Q/(eA_0) \in [1.5, 2.9, 4.4, 5.8]$. An evaluation for $d$-wave symmetry with $f(\varphi) = \cos(2\varphi)$ is shown in Fig. 3.

## IV. ASYMMETRIC PULSE

We simulate the experiment in [5] in the presence of an additional supercurrent. In this experiment, nonlinear effects in $Nb_3Sn$ lead to an asymmetric pulse shape in the material, which gives rise to an effective dc supercurrent component. Due to this current, a linear activation is possible, as described in this article, resulting in $\Omega$ oscillations of the order parameter, as well as higher odd order harmonics, which are otherwise forbidden. If an external current is applied in opposite direction, this effect may cancel and suppress again the odd orders. Following [5], we use a pulse of the shape

$$A(t) = A_0 \frac{\sin(\Omega t) + \kappa}{1 + \kappa} \mathrm{e}^{-4\log(2)\left(\frac{t - t_0}{\tau}\right)^2} \tag{42}$$

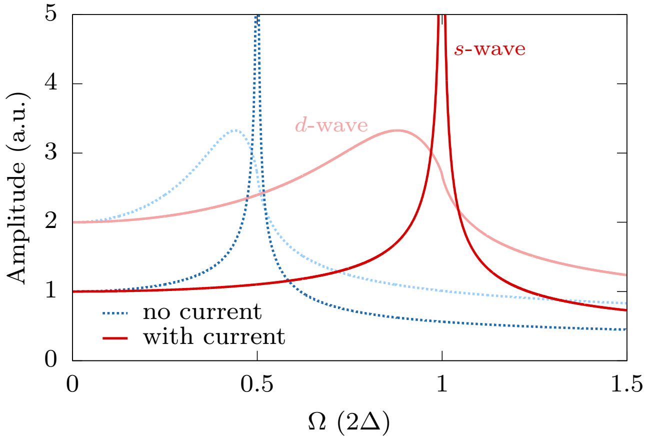


Figure 3. Amplitudes of the induced gap oscillations from Eq. (14) of the main text for $s$- and $d$-wave superconductor with $f(\varphi) = 1$ and $f(\varphi) = \cos(2\varphi)$. Resonances of the driving light with the Higgs mode appear at $2\Omega = 2\Delta$ without and at $\Omega = 2\Delta$ with supercurrent.

with frequency $\Omega$, amplitude $A_0$, full width at half maximum $\tau_p$ and a shift of the pulse center by $t_0 = \tau_p/2\sqrt{\log(1000)/\log(2)}$, such that the pulse is not cutoff starting the simulation at $t = 0$. The parameter $\kappa$ controls the asymmetry of the pulse. In the situation where an external current is present, we write

$$A_{\text{cur}} = A(t) + Q/e \tag{43}$$

with $Q$ the condensate momentum. Using this pulse shape, the Bloch equations

$$\partial_t \langle \boldsymbol{\sigma_k} \rangle = \boldsymbol{b_k} \times \langle \boldsymbol{\sigma_k} \rangle \tag{44}$$

are integrated numerically using the following parameters

$$\begin{aligned} \epsilon_{\boldsymbol{k}} &= -2t(\cos k_x + \cos k_y) - \epsilon_{\text{F}}\,, & t &= 50\text{meV}\,, & \epsilon_F &= 100\text{meV}\,, \\ 2\Delta &= 5\text{meV}\,, & eA_0 &= 0.2\,, & \Omega &= 2\text{meV}\,, \\ \tau_p &= 10\text{ps}\,, & \kappa &= 0.3\,, & Q/e &= -0.04\,. \end{aligned} \tag{45}$$

The resulting oscillations are Fourier transformed in the range $t \in [0, 30\,\text{ps}]$, where a window function is applied prior to the Fourier transform. The result is shown in Fig. 4 in the main text.


[1] T. Cea, C. Castellani, and L. Benfatto, Nonlinear optical effects and third-harmonic generation in superconductors: Cooper pairs versus Higgs mode contribution, Phys. Rev. B **93**, 180507 (2016).

[2] P. W. Anderson, Random-Phase Approximation in the Theory of Superconductivity, Phys. Rev. **112**, 1900 (1958).

[3] N. Tsuji and H. Aoki, Theory of Anderson pseudospin resonance with Higgs mode in superconductors, Phys. Rev. B **92**, 064508 (2015).

[4] S. Nakamura, Y. Iida, Y. Murotani, R. Matsunaga, H. Terai, and R. Shimano, Infrared Activation of the Higgs Mode by Supercurrent Injection in Superconducting NbN, Phys. Rev. Lett. **122**, 257001 (2019).

[5] X. Yang, C. Vaswani, C. Sundahl, M. Mootz, L. Luo, J. H. Kang, I. E. Perakis, C. B. Eom, and J. Wang, Lightwave-driven gapless superconductivity and forbidden quantum beats by terahertz symmetry breaking, Nature Photonics **13**, 707–713 (2019).
